# Supplementary material for: Bridging the Gap: Automated Analysis of Sancus
Source: arXiv:2404.09518 source file (2024-04-15)
Supplement: Supplementary file 2 [file appendix_synthesis.tex]

% !TEX root = ../main.tex
% As we anticipated in~\cref{sec:intro,sec:overview} \toolname is also able to synthesize executable code from witnesses of interfering behavior.
% For that, we provide a simple DSL that allows to specify traces of execution as a list of actions.
% We use the following notation: if an action is performed by the attacker it is preceded by \texttt{att}, otherwise it is preceded by \texttt{enc}.
% For instance, in the case of the witness graph of~\cref{fig:tree-toy}, the witnesses of interfering behavior is automatically synthesized as follows:
% %
% \begin{lstlisting}
% att: start_counting 256;
% att: create <enc_s, enc_e, data_s, data_e>;
% att: jin enc_s;
% enc: cmp s, #0;
% enc: ubr
% \end{lstlisting}
% %
% \toolname is then able to automatically substitute \lstinline|s| with the secret, compile the code to assembly, run it on the simulator, and collect the results.
% For example, it can correctly detect the difference between the two enclaves when it executes the above code: if \lstinline|s|$\ =0$ the output is $\mi{JmpOut}\ 2,\, \mi{TimerA}\ 12$, whereas if \lstinline|s|$\ =1$ leads to $\mi{JmpOut}\ 2,\, \mi{TimerA}\ 5$.

% For the synthesis of the other attacks and anomalies, we refer the interested reader to the files \texttt{attack.ml} and \texttt{attacklib.ml} in the \texttt{alvie/code/test} folder of~\cite{additionalmaterial}.
